# Supplementary material for: Folding a Small Protein Using Harmonic Linear Discriminant Analysis
Source: arXiv:1808.07895 source file (2018-08-23)
Supplement: Supplementary file 1 [file Supplementary_Materials.pdf]

# Supplementary Materials

Dan Mendels[1,2], GiovanniMaria Piccini[1,2], Z. Faidon Brotzakis[1,2], Yi I. Yang[1,2], and Michele Parrinello[1,2]

[1]Department of Chemistry and Applied Biosciences, ETH Zurich, c/o USI Campus, Via Giuseppe Buffi 13, CH-6900, Lugano, Ticino, Switzerland
[2]Facoltá di Informatica, Istituto di Scienze Computazionali, Universitá della Svizzera italiana (USI), Via Giuseppe Buffi 13, CH-6900, Lugano, Ticino, Switzerland

## Weights obtained using the HLDA for each of the descriptor sets

Table 1: HLDA coefficients for descriptor set $D_1$. $d_1, ..., d_6$ correspond to distances between atom sites located on the protein's backbone while $d_7, ..., d_{12}$ correspond to distances between atom sites located on the protein's side chains.

| | $d_1$ | $d_2$ | $d_3$ | $d_4$ | $d_5$ | $d_6$ |
|---|---|---|---|---|---|---|
| **W** | 0.2811 | 0.7997 | 0.5035 | -0.0955 | 0.0693 | 0.0072 |

| | $d_7$ | $d_8$ | $d_9$ | $d_{10}$ | $d_{11}$ | $d_{12}$ |
|---|---|---|---|---|---|---|
| **W** | -0.0097 | 0.0033 | 0.0056 | 0.1003 | 0.0355 | -0.0496 |

Table 2: HLDA coefficients for descriptor set $D_2$. $d_1, ..., d_6$ correspond to contacts between atom sites located on the protein's backbone.

| | $d_1$ | $d_2$ | $d_3$ | $d_4$ | $d_5$ | $d_6$ |
|---|---|---|---|---|---|---|
| **W** | 0.6188 | 0.5975 | 0.5045 | -0.0708 | 0.0217 | 0.0140 |

Table 3: HLDA coefficients for descriptor set $D_3$. $d_1, ..., d_9$ correspond to $\alpha\beta$ similarity functions of the proteins 9 $\phi$ dihedral angles while $d_{10} - d_{18}$ correspond to $\alpha\beta$ similarity functions of the proteins 9 $\psi$ dihedral angles.

| | $d_1$ | $d_2$ | $d_3$ | $d_4$ | $d_5$ | $d_6$ | $d_7$ | $d_8$ | $d_9$ |
|---|---|---|---|---|---|---|---|---|---|
| **W** | 0.0007 | 0.1050 | 0.2980 | 0.0815 | 0.0865 | -0.3759 | 0.0038 | 0.0234 | 0.0055 |
| | $d_{10}$ | $d_{11}$ | $d_{12}$ | $d_{13}$ | $d_{14}$ | $d_{15}$ | $d_{16}$ | $d_{17}$ | $d_{18}$ |
| **W** | 0.0008 | -0.3164 | -0.1921 | -0.6113 | -0.2871 | -0.3717 | -0.0699 | -0.0883 | -0.0108 |

# Indices of atoms used for constructing the descriptor sets

Table 4: Atom serial numbers used for the descriptor set $D_1$. See atom identity in table list below. $d_1, ..., d_6$ correspond to distances between atom sites located on the protein's backbone while $d_7, ..., d_{12}$ correspond to distances between atom sites located on the protein's side chains.

| | $d_1$ | $d_2$ | $d_3$ | $d_4$ | $d_5$ | $d_6$ |
|---|---|---|---|---|---|---|
| atom1 | 23 | 120 | 56 | 56 | 87 | 72 |
| atom2 | 149 | 46 | 101 | 108 | 101 | 87 |
| | $d_7$ | $d_8$ | $d_9$ | $d_{10}$ | $d_{11}$ | $d_{12}$ |
| atom1 | 15 | 15 | 15 | 36 | 36 | 112 |
| atom2 | 36 | 112 | 140 | 112 | 140 | 140 |

Table 5: Atom serial numbers used for the descriptor set $D_2$ and the corresponding switching function parameters used for the contacts in $D_2$. For all contacts the Plumed rational switching function was used with exponents $n = 6$ and $m = 8$. See atom identity in table list below.

| Contact num. | Atom1 | Atom2 | $R_0$ | $D_0$ |
|---|---|---|---|---|
| 1 | 23 | 149 | 0.3 | 0 |
| 2 | 120 | 46 | 0.3 | 0 |
| 3 | 56 | 101 | 0.3 | 0 |
| 4 | 56 | 108 | 0.3 | 0 |
| 5 | 87 | 101 | 0.15 | 0.08 |
| 6 | 72 | 87 | 0.12 | 0.17 |

Table 6: Reference angles utilized for the $\alpha\beta$ similarity functions used for the descriptor set $D_3$.

| Descriptor num. | Dihederal angle | Reference (rad.) |
|---|---|---|
| $d_1$ | $\Phi_2$ | $-1.938$ |
| $d_2$ | $\Phi_3$ | $-1.65$ |
| $d_3$ | $\Phi_4$ | $-1.295$ |
| $d_4$ | $\Phi_5$ | $-1.413$ |
| $d_5$ | $\Phi_6$ | 1.59 |
| $d_6$ | $\Phi_7$ | 1.428 |
| $d_7$ | $\Phi_8$ | $-2.08$ |
| $d_8$ | $\Phi_9$ | $-1.557$ |
| $d_9$ | $\Phi_{10}$ | $-1.938$ |
| $d_{10}$ | $\Psi_1$ | 2.756 |
| $d_{11}$ | $\Psi_2$ | 2.18 |
| $d_{12}$ | $\Psi_3$ | 1.99 |
| $d_{13}$ | $\Psi_4$ | $-0.35$ |
| $d_{14}$ | $\Psi_5$ | $-0.723$ |
| $d_{15}$ | $\Psi_6$ | $-0.39$ |
| $d_{16}$ | $\Psi_7$ | 0.429 |
| $d_{17}$ | $\Psi_8$ | 2.48 |
| $d_{18}$ | $\Psi_9$ | 2.19 |

Table 7: Topology table used for the simulations

| | | | | | | | | | | |
|---|---|---|---|---|---|---|---|---|---|---|
| ATOM | 1 | N | TYR | 1 | 10.866 | -13.579 | -19.419 | 0 | 0 | N |
| ATOM | 2 | HT1 | TYR | 1 | 11.193 | -12.732 | -19.864 | 0 | 0 | H |
| ATOM | 3 | HT2 | TYR | 1 | 10.051 | -13.955 | -19.882 | 0 | 0 | H |
| ATOM | 4 | HT3 | TYR | 1 | 11.638 | -14.227 | -19.484 | 0 | 0 | H |
| ATOM | 5 | CA | TYR | 1 | 10.585 | -13.392 | -18.05 | 0 | 0 | C |
| ATOM | 6 | HA | TYR | 1 | 9.961 | -12.507 | -17.925 | 0 | 0 | H |
| ATOM | 7 | CB | TYR | 1 | 9.69 | -14.502 | -17.442 | 0 | 0 | C |
| ATOM | 8 | HB1 | TYR | 1 | 8.667 | -14.457 | -17.815 | 0 | 0 | H |
| ATOM | 9 | HB2 | TYR | 1 | 10.108 | -15.453 | -17.771 | 0 | 0 | H |
| ATOM | 10 | CG | TYR | 1 | 9.672 | -14.561 | -15.96 | 0 | 0 | C |
| ATOM | 11 | CD1 | TYR | 1 | 10.278 | -15.544 | -15.203 | 0 | 0 | C |
| ATOM | 12 | HD1 | TYR | 1 | 10.641 | -16.451 | -15.665 | 0 | 0 | H |
| ATOM | 13 | CE1 | TYR | 1 | 10.361 | -15.429 | -13.778 | 0 | 0 | C |
| ATOM | 14 | HE1 | TYR | 1 | 10.902 | -16.131 | -13.161 | 0 | 0 | H |
| ATOM | 15 | CZ | TYR | 1 | 9.696 | -14.34 | -13.177 | 0 | 0 | C |
| ATOM | 16 | OH | TYR | 1 | 9.725 | -14.18 | -11.849 | 0 | 0 | O |
| ATOM | 17 | HH | TYR | 1 | 9.356 | -13.345 | -11.552 | 0 | 0 | H |
| ATOM | 18 | CD2 | TYR | 1 | 9.071 | -13.439 | -15.334 | 0 | 0 | C |
| ATOM | 19 | HD2 | TYR | 1 | 8.692 | -12.62 | -15.928 | 0 | 0 | H |
| ATOM | 20 | CE2 | TYR | 1 | 9.103 | -13.348 | -13.971 | 0 | 0 | C |
| ATOM | 21 | HE2 | TYR | 1 | 8.718 | -12.403 | -13.617 | 0 | 0 | H |
| ATOM | 22 | C | TYR | 1 | 11.834 | -12.912 | -17.26 | 0 | 0 | C |
| ATOM | 23 | O | TYR | 1 | 12.124 | -11.729 | -17.301 | 0 | 0 | O |
| ATOM | 24 | N | TYR | 2 | 12.696 | -13.817 | -16.752 | 0 | 0 | N |
| ATOM | 25 | HN | TYR | 2 | 12.518 | -14.809 | -16.816 | 0 | 0 | H |
| ATOM | 26 | CA | TYR | 2 | 13.807 | -13.413 | -15.897 | 0 | 0 | C |
| ATOM | 27 | HA | TYR | 2 | 14.119 | -12.412 | -16.193 | 0 | 0 | H |
| ATOM | 28 | CB | TYR | 2 | 13.208 | -13.199 | -14.475 | 0 | 0 | C |
| ATOM | 29 | HB1 | TYR | 2 | 12.771 | -12.201 | -14.449 | 0 | 0 | H |
| ATOM | 30 | HB2 | TYR | 2 | 12.274 | -13.726 | -14.277 | 0 | 0 | H |
| ATOM | 31 | CG | TYR | 2 | 14.19 | -13.332 | -13.315 | 0 | 0 | C |
| ATOM | 32 | CD1 | TYR | 2 | 14.285 | -14.61 | -12.72 | 0 | 0 | C |
| ATOM | 33 | HD1 | TYR | 2 | 13.685 | -15.436 | -13.071 | 0 | 0 | H |
| ATOM | 34 | CE1 | TYR | 2 | 15.276 | -14.923 | -11.746 | 0 | 0 | C |
| ATOM | 35 | HE1 | TYR | 2 | 15.348 | -15.859 | -11.212 | 0 | 0 | H |
| ATOM | 36 | CZ | TYR | 2 | 16.196 | -13.922 | -11.374 | 0 | 0 | C |
| ATOM | 37 | OH | TYR | 2 | 17.154 | -14.147 | -10.37 | 0 | 0 | O |
| ATOM | 38 | HH | TYR | 2 | 17.59 | -13.353 | -10.052 | 0 | 0 | H |
| ATOM | 39 | CD2 | TYR | 2 | 15.127 | -12.38 | -12.935 | 0 | 0 | C |
| ATOM | 40 | HD2 | TYR | 2 | 15.057 | -11.419 | -13.422 | 0 | 0 | H |
| ATOM | 41 | CE2 | TYR | 2 | 16.082 | -12.629 | -11.957 | 0 | 0 | C |
| ATOM | 42 | HE2 | TYR | 2 | 16.792 | -11.85 | -11.722 | 0 | 0 | H |
| ATOM | 43 | C | TYR | 2 | 14.991 | -14.435 | -15.898 | 0 | 0 | C |

| | | | | | | | | | | |
|---|---|---|---|---|---|---|---|---|---|---|
| ATOM | 44 | O | TYR | 2 | 14.944 | -15.604 | -16.118 | 0 | 0 | O |
| ATOM | 45 | N | ASP | 3 | 16.121 | -13.807 | -15.693 | 0 | 0 | N |
| ATOM | 46 | HN | ASP | 3 | 16.126 | -12.798 | -15.744 | 0 | 0 | H |
| ATOM | 47 | CA | ASP | 3 | 17.448 | -14.337 | -15.687 | 0 | 0 | C |
| ATOM | 48 | HA | ASP | 3 | 17.448 | -15.371 | -15.342 | 0 | 0 | H |
| ATOM | 49 | CB | ASP | 3 | 18.039 | -14.416 | -17.125 | 0 | 0 | C |
| ATOM | 50 | HB1 | ASP | 3 | 17.372 | -15.163 | -17.555 | 0 | 0 | H |
| ATOM | 51 | HB2 | ASP | 3 | 17.972 | -13.505 | -17.719 | 0 | 0 | H |
| ATOM | 52 | CG | ASP | 3 | 19.468 | -15.042 | -17.253 | 0 | 0 | C |
| ATOM | 53 | OD1 | ASP | 3 | 20.519 | -14.33 | -17.392 | 0 | 0 | O |
| ATOM | 54 | OD2 | ASP | 3 | 19.48 | -16.31 | -17.217 | 0 | 0 | O |
| ATOM | 55 | C | ASP | 3 | 18.257 | -13.555 | -14.672 | 0 | 0 | C |
| ATOM | 56 | O | ASP | 3 | 18.091 | -12.314 | -14.636 | 0 | 0 | O |
| ATOM | 57 | N | PRO | 4 | 19.084 | -14.145 | -13.763 | 0 | 0 | N |
| ATOM | 58 | CD | PRO | 4 | 19.656 | -15.423 | -13.846 | 0 | 0 | C |
| ATOM | 59 | HD1 | PRO | 4 | 18.944 | -16.234 | -13.701 | 0 | 0 | H |
| ATOM | 60 | HD2 | PRO | 4 | 20.162 | -15.551 | -14.803 | 0 | 0 | H |
| ATOM | 61 | CA | PRO | 4 | 19.754 | -13.38 | -12.71 | 0 | 0 | C |
| ATOM | 62 | HA | PRO | 4 | 18.957 | -13.004 | -12.068 | 0 | 0 | H |
| ATOM | 63 | CB | PRO | 4 | 20.441 | -14.337 | -11.788 | 0 | 0 | C |
| ATOM | 64 | HB1 | PRO | 4 | 19.727 | -14.607 | -11.01 | 0 | 0 | H |
| ATOM | 65 | HB2 | PRO | 4 | 21.354 | -13.878 | -11.41 | 0 | 0 | H |
| ATOM | 66 | CG | PRO | 4 | 20.738 | -15.467 | -12.769 | 0 | 0 | C |
| ATOM | 67 | HG1 | PRO | 4 | 20.829 | -16.421 | -12.249 | 0 | 0 | H |
| ATOM | 68 | HG2 | PRO | 4 | 21.722 | -15.303 | -13.209 | 0 | 0 | H |
| ATOM | 69 | C | PRO | 4 | 20.627 | -12.232 | -13.162 | 0 | 0 | C |
| ATOM | 70 | O | PRO | 4 | 21.512 | -12.437 | -14.059 | 0 | 0 | O |
| ATOM | 71 | N | GLU | 5 | 20.56 | -11.005 | -12.571 | 0 | 0 | N |
| ATOM | 72 | HN | GLU | 5 | 20.029 | -10.824 | -11.73 | 0 | 0 | H |
| ATOM | 73 | CA | GLU | 5 | 21.387 | -9.89 | -12.993 | 0 | 0 | C |
| ATOM | 74 | HA | GLU | 5 | 21.413 | -9.738 | -14.072 | 0 | 0 | H |
| ATOM | 75 | CB | GLU | 5 | 20.902 | -8.514 | -12.434 | 0 | 0 | C |
| ATOM | 76 | HB1 | GLU | 5 | 21.35 | -7.747 | -13.066 | 0 | 0 | H |
| ATOM | 77 | HB2 | GLU | 5 | 19.862 | -8.536 | -12.761 | 0 | 0 | H |
| ATOM | 78 | CG | GLU | 5 | 20.902 | -8.011 | -10.919 | 0 | 0 | C |
| ATOM | 79 | HG1 | GLU | 5 | 21.917 | -8.054 | -10.523 | 0 | 0 | H |
| ATOM | 80 | HG2 | GLU | 5 | 20.564 | -6.976 | -10.867 | 0 | 0 | H |
| ATOM | 81 | CD | GLU | 5 | 20.029 | -8.793 | -10.003 | 0 | 0 | C |
| ATOM | 82 | OE1 | GLU | 5 | 18.877 | -8.411 | -9.77 | 0 | 0 | O |

| | | | | | | | | | | |
|---|---|---|---|---|---|---|---|---|---|---|
| ATOM | 83 | OE2 | GLU | 5 | 20.479 | -9.887 | -9.556 | 0 | 0 | O |
| ATOM | 84 | C | GLU | 5 | 22.839 | -10.033 | -12.585 | 0 | 0 | C |
| ATOM | 85 | O | GLU | 5 | 23.695 | -9.44 | -13.236 | 0 | 0 | O |
| ATOM | 86 | N | THR | 6 | 23.142 | -10.755 | -11.482 | 0 | 0 | N |
| ATOM | 87 | HN | THR | 6 | 22.304 | -10.998 | -10.973 | 0 | 0 | H |
| ATOM | 88 | CA | THR | 6 | 24.477 | -11.132 | -11.001 | 0 | 0 | C |
| ATOM | 89 | HA | THR | 6 | 25.08 | -10.271 | -11.289 | 0 | 0 | H |
| ATOM | 90 | CB | THR | 6 | 24.465 | -11.48 | -9.534 | 0 | 0 | C |
| ATOM | 91 | HB | THR | 6 | 25.431 | -11.857 | -9.198 | 0 | 0 | H |
| ATOM | 92 | OG1 | THR | 6 | 23.493 | -12.508 | -9.226 | 0 | 0 | O |
| ATOM | 93 | HG1 | THR | 6 | 23.487 | -12.603 | -8.271 | 0 | 0 | H |
| ATOM | 94 | CG2 | THR | 6 | 24.107 | -10.358 | -8.52 | 0 | 0 | C |
| ATOM | 95 | HG21 | THR | 6 | 23.022 | -10.258 | -8.502 | 0 | 0 | H |
| ATOM | 96 | HG22 | THR | 6 | 24.432 | -10.71 | -7.541 | 0 | 0 | H |
| ATOM | 97 | HG23 | THR | 6 | 24.648 | -9.464 | -8.831 | 0 | 0 | H |
| ATOM | 98 | C | THR | 6 | 25.113 | -12.294 | -11.782 | 0 | 0 | C |
| ATOM | 99 | O | THR | 6 | 26.337 | -12.547 | -11.791 | 0 | 0 | O |
| ATOM | 100 | N | GLY | 7 | 24.31 | -13.105 | -12.495 | 0 | 0 | N |
| ATOM | 101 | HN | GLY | 7 | 23.329 | -12.888 | -12.39 | 0 | 0 | H |
| ATOM | 102 | CA | GLY | 7 | 24.749 | -14.128 | -13.464 | 0 | 0 | C |
| ATOM | 103 | HA1 | GLY | 7 | 25.572 | -13.678 | -14.019 | 0 | 0 | H |
| ATOM | 104 | HA2 | GLY | 7 | 23.947 | -14.451 | -14.129 | 0 | 0 | H |
| ATOM | 105 | C | GLY | 7 | 25.326 | -15.45 | -12.875 | 0 | 0 | C |
| ATOM | 106 | O | GLY | 7 | 25.155 | -16.488 | -13.495 | 0 | 0 | O |
| ATOM | 107 | N | THR | 8 | 25.98 | -15.436 | -11.759 | 0 | 0 | N |
| ATOM | 108 | HN | THR | 8 | 26.047 | -14.555 | -11.269 | 0 | 0 | H |
| ATOM | 109 | CA | THR | 8 | 26.568 | -16.621 | -11.092 | 0 | 0 | C |
| ATOM | 110 | HA | THR | 8 | 26.946 | -17.369 | -11.789 | 0 | 0 | H |
| ATOM | 111 | CB | THR | 8 | 27.695 | -16.186 | -10.141 | 0 | 0 | C |
| ATOM | 112 | HB | THR | 8 | 27.837 | -16.842 | -9.282 | 0 | 0 | H |
| ATOM | 113 | OG1 | THR | 8 | 27.514 | -14.818 | -9.791 | 0 | 0 | O |
| ATOM | 114 | HG1 | THR | 8 | 28.258 | -14.701 | -9.196 | 0 | 0 | H |
| ATOM | 115 | CG2 | THR | 8 | 29.014 | -16.267 | -10.929 | 0 | 0 | C |
| ATOM | 116 | HG21 | THR | 8 | 29.75 | -15.685 | -10.374 | 0 | 0 | H |
| ATOM | 117 | HG22 | THR | 8 | 29.175 | -17.312 | -11.192 | 0 | 0 | H |
| ATOM | 118 | HG23 | THR | 8 | 28.931 | -15.643 | -11.819 | 0 | 0 | H |
| ATOM | 119 | C | THR | 8 | 25.537 | -17.419 | -10.283 | 0 | 0 | C |
| ATOM | 120 | O | THR | 8 | 25.829 | -18.602 | -10.05 | 0 | 0 | O |
| ATOM | 121 | N | TRP | 9 | 24.445 | -16.806 | -9.902 | 0 | 0 | N |
| ATOM | 122 | HN | TRP | 9 | 24.271 | -15.843 | -10.152 | 0 | 0 | H |

| | | | | | | | | | | |
|---|---|---|---|---|---|---|---|---|---|---|
| ATOM | 123 | CA | TRP | 9 | 23.44 | -17.489 | -8.982 | 0 | 0 | C |
| ATOM | 124 | HA | TRP | 9 | 23.628 | -18.558 | -9.082 | 0 | 0 | H |
| ATOM | 125 | CB | TRP | 9 | 23.627 | -17.159 | -7.442 | 0 | 0 | C |
| ATOM | 126 | HB1 | TRP | 9 | 23.118 | -16.197 | -7.391 | 0 | 0 | H |
| ATOM | 127 | HB2 | TRP | 9 | 23.169 | -17.951 | -6.85 | 0 | 0 | H |
| ATOM | 128 | CG | TRP | 9 | 25.019 | -16.966 | -6.887 | 0 | 0 | C |
| ATOM | 129 | CD1 | TRP | 9 | 25.842 | -17.957 | -6.644 | 0 | 0 | C |
| ATOM | 130 | HD1 | TRP | 9 | 25.591 | -19 | -6.772 | 0 | 0 | H |
| ATOM | 131 | NE1 | TRP | 9 | 27.009 | -17.615 | -6.073 | 0 | 0 | N |
| ATOM | 132 | HE1 | TRP | 9 | 27.698 | -18.313 | -5.833 | 0 | 0 | H |
| ATOM | 133 | CE2 | TRP | 9 | 27.139 | -16.27 | -6.163 | 0 | 0 | C |
| ATOM | 134 | CD2 | TRP | 9 | 25.841 | -15.795 | -6.596 | 0 | 0 | C |
| ATOM | 135 | CE3 | TRP | 9 | 25.747 | -14.404 | -6.911 | 0 | 0 | C |
| ATOM | 136 | HE3 | TRP | 9 | 24.813 | -14.018 | -7.293 | 0 | 0 | H |
| ATOM | 137 | CZ3 | TRP | 9 | 26.778 | -13.516 | -6.497 | 0 | 0 | C |
| ATOM | 138 | HZ3 | TRP | 9 | 26.607 | -12.502 | -6.826 | 0 | 0 | H |
| ATOM | 139 | CZ2 | TRP | 9 | 28.162 | -15.334 | -5.771 | 0 | 0 | C |
| ATOM | 140 | HZ2 | TRP | 9 | 29.145 | -15.61 | -5.417 | 0 | 0 | H |
| ATOM | 141 | CH2 | TRP | 9 | 28.014 | -13.964 | -6.063 | 0 | 0 | C |
| ATOM | 142 | HH2 | TRP | 9 | 28.859 | -13.336 | -5.824 | 0 | 0 | H |
| ATOM | 143 | C | TRP | 9 | 21.935 | -17.395 | -9.224 | 0 | 0 | C |
| ATOM | 144 | O | TRP | 9 | 21.396 | -16.293 | -9.619 | 0 | 0 | O |
| ATOM | 145 | C | TYR | 10 | 19.108 | -18.996 | -7.571 | 0 | 0 | C |
| ATOM | 146 | OT1 | TYR | 10 | 19.422 | -18.26 | -6.552 | 0 | 0 | O |
| ATOM | 147 | OT2 | TYR | 10 | 18.274 | -19.868 | -7.393 | 0 | 0 | O |
| ATOM | 148 | N | TYR | 10 | 21.221 | -18.465 | -8.793 | 0 | 0 | N |
| ATOM | 149 | HN | TYR | 10 | 21.745 | -19.256 | -8.445 | 0 | 0 | H |
| ATOM | 150 | CA | TYR | 10 | 19.72 | -18.48 | -8.832 | 0 | 0 | C |
| ATOM | 151 | HA | TYR | 10 | 19.375 | -17.501 | -9.165 | 0 | 0 | H |
| ATOM | 152 | CB | TYR | 10 | 19.346 | -19.4 | -10.061 | 0 | 0 | C |
| ATOM | 153 | HB1 | TYR | 10 | 20.104 | -19.253 | -10.83 | 0 | 0 | H |
| ATOM | 154 | HB2 | TYR | 10 | 19.232 | -20.419 | -9.692 | 0 | 0 | H |
| ATOM | 155 | CG | TYR | 10 | 18.032 | -19.118 | -10.721 | 0 | 0 | C |
| ATOM | 156 | CD1 | TYR | 10 | 17.963 | -18.24 | -11.724 | 0 | 0 | C |
| ATOM | 157 | HD1 | TYR | 10 | 18.914 | -17.792 | -11.968 | 0 | 0 | H |
| ATOM | 158 | CE1 | TYR | 10 | 16.745 | -18.07 | -12.458 | 0 | 0 | C |
| ATOM | 159 | HE1 | TYR | 10 | 16.608 | -17.374 | -13.272 | 0 | 0 | H |
| ATOM | 160 | CZ | TYR | 10 | 15.627 | -18.721 | -11.944 | 0 | 0 | C |
| ATOM | 161 | OH | TYR | 10 | 14.463 | -18.416 | -12.5 | 0 | 0 | O |
| ATOM | 162 | HH | TYR | 10 | 13.72 | -18.487 | -11.896 | 0 | 0 | H |
| ATOM | 163 | CD2 | TYR | 10 | 16.829 | -19.75 | -10.203 | 0 | 0 | C |
| ATOM | 164 | HD2 | TYR | 10 | 16.927 | -20.366 | -9.321 | 0 | 0 | H |
| ATOM | 165 | CE2 | TYR | 10 | 15.617 | -19.561 | -10.85 | 0 | 0 | C |
| ATOM | 166 | HE2 | TYR | 10 | 14.707 | -19.947 | -10.415 | 0 | 0 | H |

## HLDA code availability

The HLDA code providing the coefficients of the linear combination is now also available in a development version for PLUMED2 at the following URL: `https://github.com/helloyesterday/plumed2_HLDA`. We kindly acknowledge Dr. Y. I. Yang for implementing this first version of the code for PLUMED2.
